# Supplementary material for: Precise measurements of torque in von Karman swirling flow driven by a bladed disk
Source: arXiv:1801.01845 source file (2018-01-05)
Supplement: Supplementary file 1 [file Supplemetmater.pdf]

# Supplemental Material:
# Precise torque measurements in von Karman swirling flow driven by a bladed disk

Aryesh Mukherjee[1], Sergei Lukaschuk[2], Yuri Burnishev[1], Gregory Falkovich[1], and Victor Steinberg[1,3]
[1] *Department of Physics of Complex Systems, Weizmann Institute of Science, Rehovot 76100, Israel,* [2] *Permanent address: University of Hull, Hull, GB,* [3] *The Rakah Institute of Physics, the Hebrew University of Jerusalem, Jerusalem 91904, Israel*

[1] F. Ravelet, A. Chiffaudel, and F. Daviaud, Supercritical transition to turbulence in an inertially driven von Karman closed flow, *J. Fluid Mech.* **601**, 339 (2008).

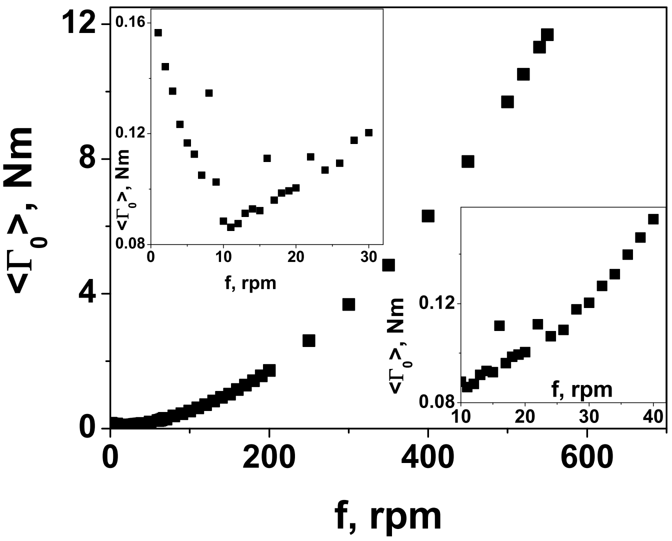


**Fig.** 1SM: The average torque $\langle\Gamma_0\rangle$ as a function of rotation frequency $f$ in a wide range of its variations down to 1 rpm for water at $T = 45°C$ for the first setup with two counter-rotating bladed disks. Insets: the same data at higher resolution at low $f$.

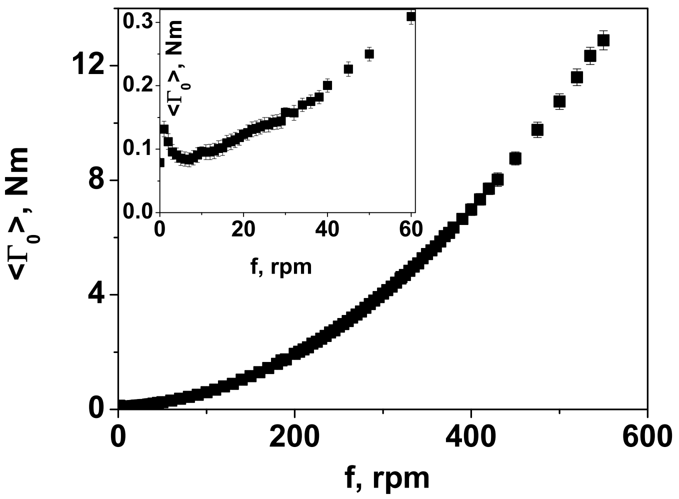


**Fig.** 2SM: The average torque $\langle\Gamma_0\rangle$ as a function of rotation frequency $f$ in a wide range of its variations down to 1 rpm for water-glycerin solution of 50% w/w glycerin concentration at $T = 24°C$ for the first setup with two counter-rotating bladed disks. Inset: the same data at higher resolution at low $f$.

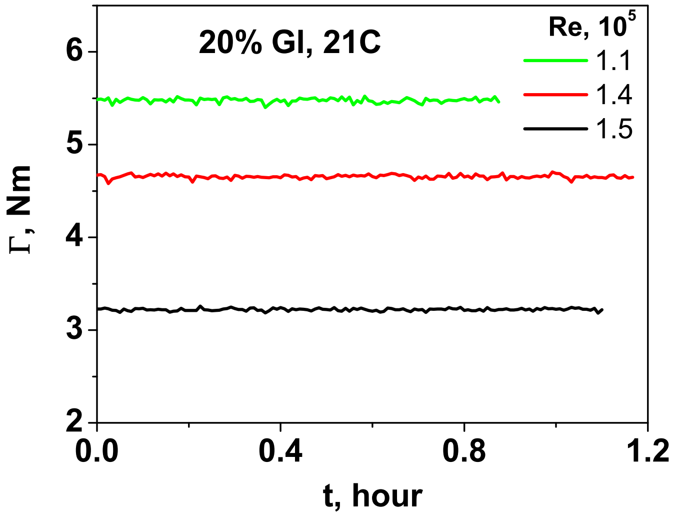


**Fig.** 3SM: (Color online) Time series of torque $\Gamma(t)$ in the constant $\Omega$ regime for water-glycerin solution of 20% w/w concentration and $T = 21°C$ at various $Re$: (a) $1.1 \times 10^5$; (b) $1.4 \times 10^5$; (c) $1.5 \times 10^5$.

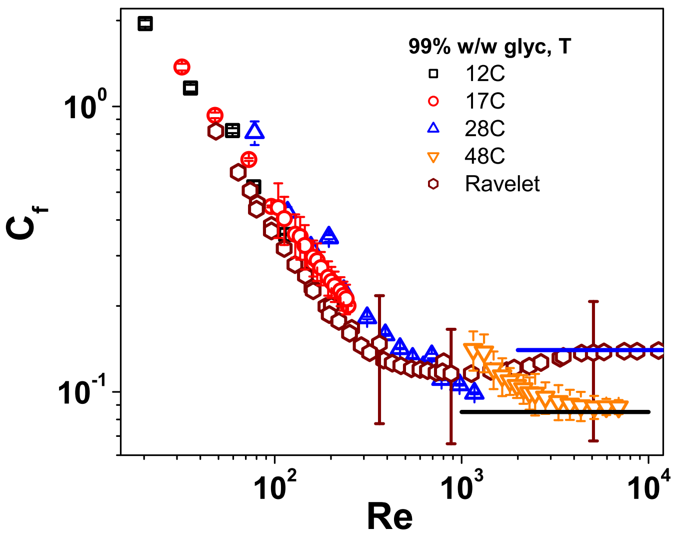


**Fig.** 4SM: (Color online) Comparison of the friction coefficient $C_f$with error bars versus $Re$ for water-glycerin solution of 99% w/w glycerin concentration at various temperatures for the first setup and of the data with large error bars from Ref. [1]. Solid black at $C_f \simeq 0.085$ and solid blue at $C_f \simeq 0.14$ lines are to indicate a constant values of $C_f$ in a fully developed turbulent state for our data and for the data from Ref. [1], respectively.

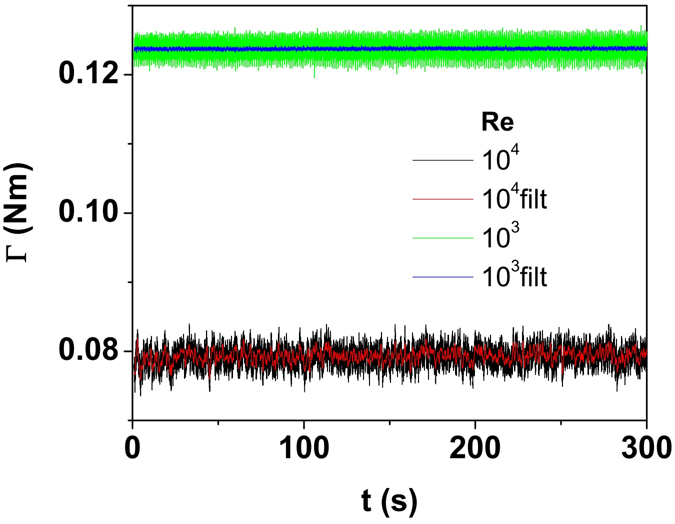


**Fig.** 5SM: (Color online) Time series of $Gamma$ for water-glycerin solutions with two w/w glycerin concentrations and $Re$ for the second setup with one bladed disk: 50%, $Re = 10^4$ and 85%, $Re = 10^3$.

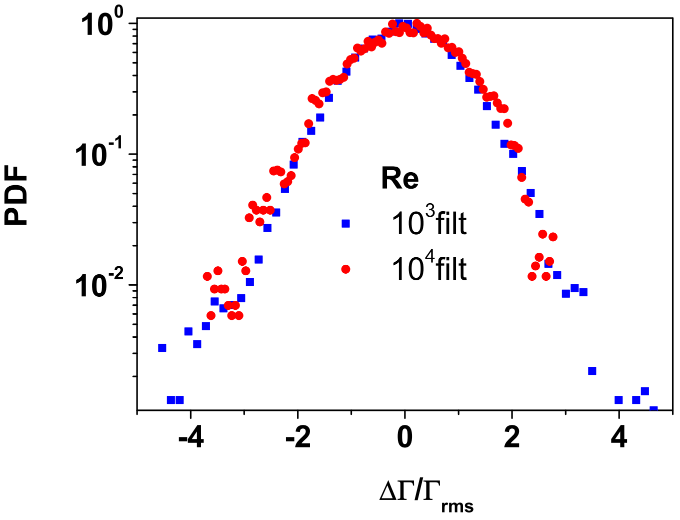


**Fig.** 6SM: (Color online) PDFs of $\delta\Gamma/\Gamma_{rms}$ for water-glycerin solutions with two w/w glycerin concentrations and $Re$ for the second setup with one bladed disk: 50%, $Re = 10^4$ and 85%, $Re = 10^3$.

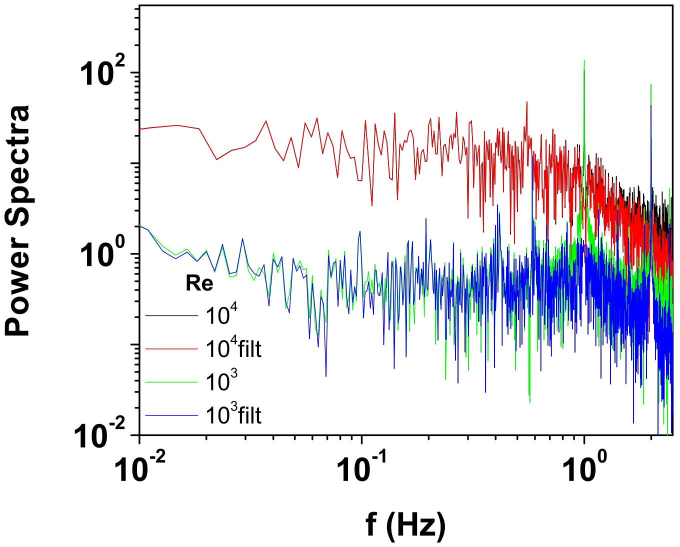


**Fig.** 7SM: (Color online) Power spectra of torque $\Gamma$ for water-glycerin solutions with two w/w glycerin concentrations and $Re$ for the second setup with one bladed disk: 50%, $Re = 10^4$ and 85%, $Re = 10^3$.
